# Supplementary material for: Robust Graph Learning Against Adversarial Evasion Attacks via Prior-Free Diffusion-Based Structure Purification
Source: arXiv:2502.05000 source file (2025-02-07)
Supplement: Supplementary file 1 [file 7.appendix_algorithm.tex]

\section{Algorithm of \ModelName}\label{appendix:algorithm}
The whole purification process of \ModelName is presented in Algorithm~\ref{algorithm_\ModelName}

\begin{algorithm}
\caption{Overall purification process of \ModelName.}
\label{algorithm:\ModelName}
\KwIn {Attacked graph adjacency matrix $A_{adv}$; Pre-trained GNN classifier $c_{\hat{\theta}}$; Pre-trained graph diffusion model $\phi_{\theta}$; Number of diffusion steps $T$; Hyperparameters $k, \lambda$.}
\KwOut{Purified adjacency matrix $\hat{A}$.}
\BlankLine
\tcp{LID Score}
Obtain the adversarial score of each edge $\Lambda(A)=\Gamma \Gamma^{T}$, with $\Gamma \leftarrow$ Eq.~(\ref{equation_lid_score})\;
Obtain the purification time of each edge $\hat{t}(A_{ij})\leftarrow$ Eq.~(\ref{equation_purification_time})\;
\For{$t=T,T-1,\cdots,1$}{
    \tcp{Non-Isotropic Purification}
    Establish the purification mask $M_{ij}^{(t-1)}\leftarrow$ Eq.~(\ref{equation_mask})\;
    Obtain the forward noisy adjacency matrix $A_{adv}^{(t-1)}$ and the predict adjacency matrix $\hat{G}^{(t-1)}$ at time $t-1$ using $\phi_{\theta}$\;
    Update the predict adjacency matrix  $\hat{A}^{(t-1)}\leftarrow$ Eq.~(\ref{equation_non_isotropic_purification})

    \tcp{Graph Transfer Entropy Guided Purification}
    Calculate the graph transfer entropy $I(\hat{G}^{t-1}; G_{adv}| \hat{G}_{t})\leftarrow$ Eq.~(\ref{transfer entropy})~(\ref{graph_entropy})~(\ref{graph_joint_entropy})\;

    Guide the generation process $\hat{A}^{(t-1)}\leftarrow$ Eq.~(\ref{equation_guide_generation})
}
Obtain the $\hat{A}^{(0)}$ as the purified ajacency matrix $\hat{A}$
\end{algorithm}
